# Supplementary material for: Manipulating Core-Excitations in Molecules by X-ray Cavities
Source: arXiv:2101.01838 source file (2021-01-06)
Supplement: Supplementary file 1 [file SI.pdf]

# Supporting Information: Manipulating Core-Excitations in Molecules by X-ray Cavities

Bing Gu,[1,*] Artur Nenov,[2,*] Francesco Segatta,[2] Marco Garavelli,[2,†] and Shaul Mukamel[1,‡]

[1] *Department of Chemistry and Department of Physics and Astronomy, University of California, Irvine, 92697, USA*

[2] *Dipartimento di Chimica Industriale "Toso Montanari", Università degli studi di Bologna, Viale del Risorgimento 4, 40136 Bologna, Italy.*

* These authors contributed equally to this work.

† marco.garavelli@unibo.it

‡ smukamel@uci.edu

**CONTENTS**

S1. Derivation of Eq. (2) S2

S2. Electronic structure simulations S3

S3. Simulations of spectra S7

S3.A. Sum-over-states expression for XANES S8

S4. Two-photon absorption S9

References S10

## S1. DERIVATION OF EQ. (2)

Under the rotating-wave and long-wavelength approximations,

$$H_{\mathrm{CM}} = \mathbf{V}^\dagger \cdot \hat{\mathbf{E}}^{(+)}(\mathbf{r}=0) + \mathrm{H.c.} \tag{S1}$$

where $\mathbf{V}$ and $\mathbf{V}^\dagger$ are, respectively, the lowering and raising dipole operator $\mathbf{V} + \mathbf{V}^\dagger = -\sum_n \boldsymbol{\mu}^{(n)}$ and $\hat{\mathbf{E}}^{(+)}(\mathbf{r})$ ($\hat{\mathbf{E}}^{(-)}(\mathbf{r})$) is the positive (negative)-frequency component of the electric field operator.

With the collective states

$$|C_{\alpha k}\rangle = \frac{1}{\sqrt{N}} \sum_k e^{ikn} |c_\alpha^{(n)}\rangle, \tag{S2}$$

for $c = e, f$ and $k = 2\pi j/N, j = 0, \cdots, N-1$, the local core-excitation states (in the many-body space) can be rewritten as

$$|c_\alpha^{(n)}\rangle = \frac{1}{\sqrt{N}} \sum_k e^{-ikn} |C_{\alpha k}\rangle \tag{S3}$$

Up to double excitations, the relevant molecular states contain $|G\rangle, |E_{\alpha k}\rangle, |F_{\beta k}\rangle, \left|e_\alpha^{(n)} e_\beta^{(m)}\right\rangle, n \neq m$. Within this subspace, inserting Eq. (S3) into the cavity-molecule coupling yields Eq. (2)

$$\begin{aligned} H_{\mathrm{CM}} =& \sum_k \sum_n \kappa_{e_\alpha g} \frac{1}{\sqrt{N}} e^{-ikn} |E_{\alpha k}\rangle \langle G| a + \sum_{\alpha,\beta} \sum_{k,k'} \sum_n \frac{1}{N} e^{-i(k-k')n} \kappa_{f_\beta e_\alpha} |F_{\beta k}\rangle \langle E_{\alpha k'}| a \\ &+ \sum_{n\neq m} \sum_{\alpha,\gamma} \kappa_{e_\alpha g} |e_\alpha^{(n)} e_\gamma^{(m)}\rangle \langle e_\gamma^{(m)}| a + \mathrm{H.c.} \\ =& \sum_\alpha \kappa_{e_\alpha g} \sqrt{N} |E_{\alpha 0}\rangle \langle G| a + \sum_{\alpha,\beta} \sum_k \kappa_{f_\beta e_\alpha} |F_{\beta k}\rangle \langle E_{\alpha k}| a + \sum_{n\neq m} \sum_{\alpha,\gamma} \kappa_{e_\alpha g} |e_\alpha^{(n)} e_\gamma^{(m)}\rangle \langle e_\gamma^{(m)}| + \mathrm{H.c.} \end{aligned} \tag{S4}$$

where $\kappa_{ji} = \sqrt{\hbar\omega_{\mathrm{c}}/2\varepsilon_0 V_{\mathrm{c}}} \langle j|\boldsymbol{\mu} \cdot \mathbf{e}_{\mathrm{c}}|i\rangle$.

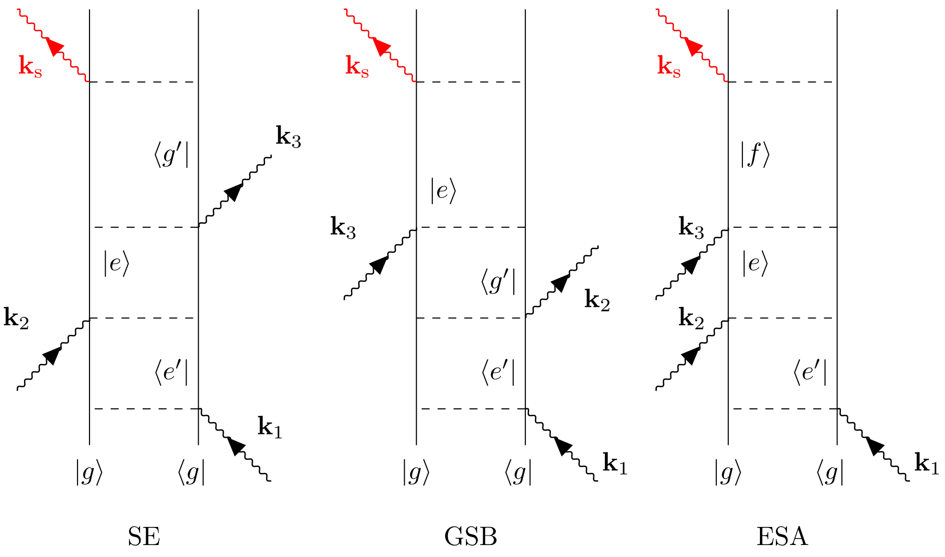


FIG. S1. Three double-sided Feynman diagrams for the 2D photon echo signal. GSB: ground state bleaching; SE: stimulated emission; ESA: excited state absorption.

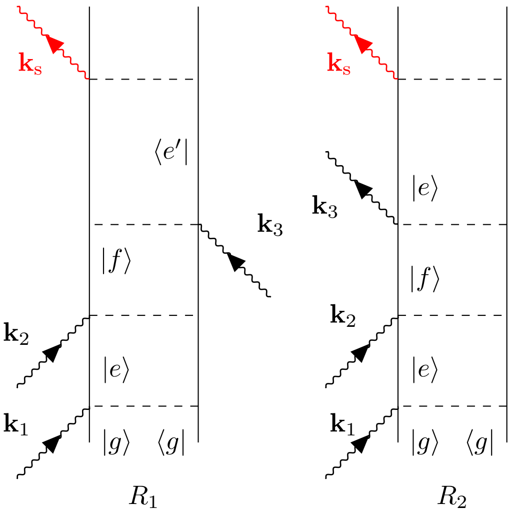


FIG. S2. Two double-sided Feynman diagrams contributing to the 2D double quantum coherence signal. The pump pulses $\mathbf{k}_1$ and $\mathbf{k}_2$ brings the system to a double-quantum coherence $|f\rangle\langle g|$.

## S2. ELECTRONIC STRUCTURE SIMULATIONS

The ground state ($g$) and the manifolds of singly ($e$) and doubly ($f$) core-excited states of 1,1-difluoroethylene cannot be computed in one shot as they are energetically separated by several hundreds of eV (carbon K-edge is around 290 eV above the ground state (GS), whereas the $f$ manifold contains states absorbing around 580 eV. This implies that a number of electronic states, irrelevant to the issue under scrutiny, are situated in between the manifolds.

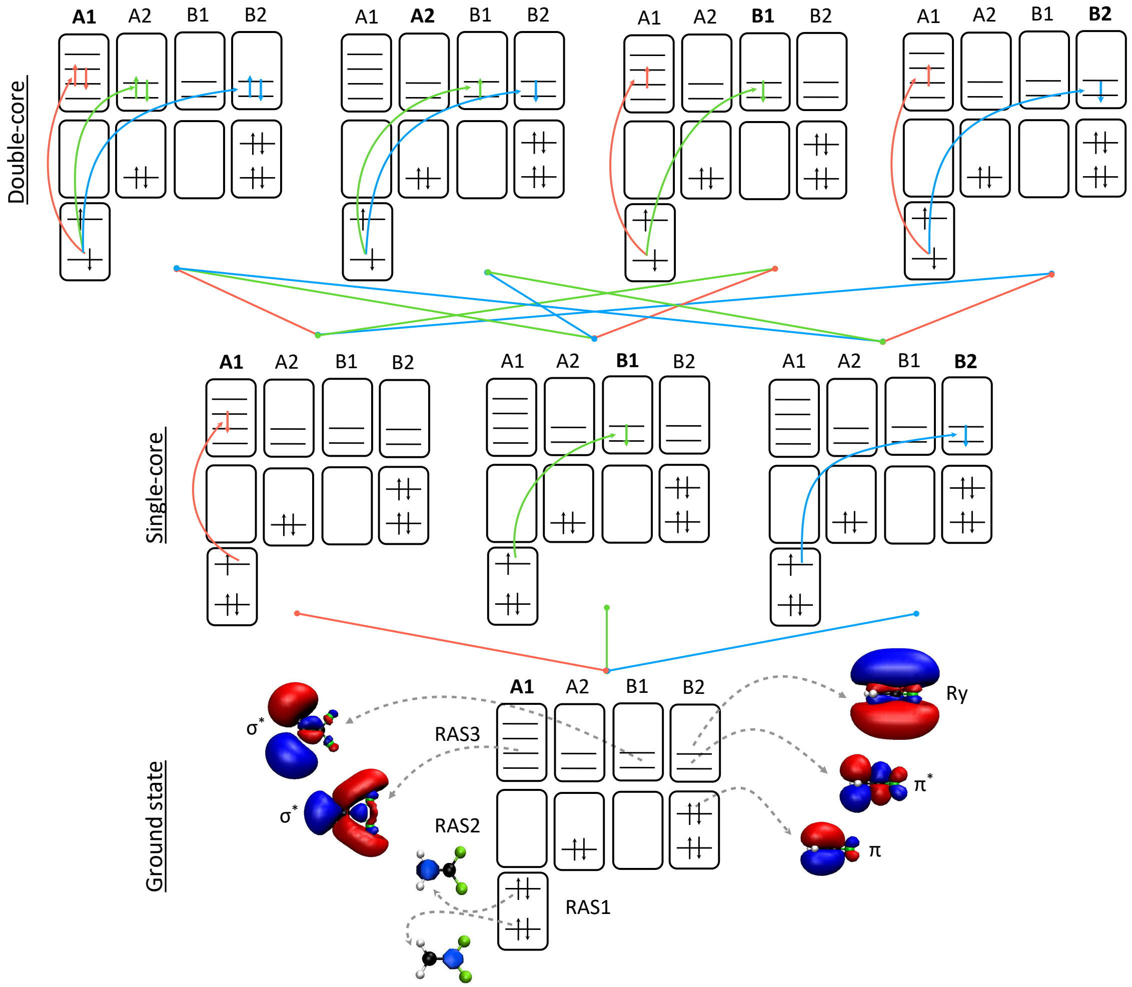


FIG. S3. Scheme showing the ground state, single- and double-core excited manifolds (grouped by symmetry) of 1,1-difluoroethylene with the restricted active space RAS(10, 2, 4; 2, 3, 10) defined in the text. The various transitions connecting the manifolds are depicted and highlighted in color according to the irreducible representation to which the orbitals involved in the corresponding $g \to e$ or $e \to f$ transition belong, namely A1 (red) B1 (green) and B2 (blue). Each of the eight electronic configurations shown requires a separate calculation, each arrow denotes a non-zero transition dipole vector between manifolds. Representative orbitals of the active space are also shown.

The strategy to target single- and double-core excitations used here is based on the restricted active space self consistent field (RASSCF) approach [1] from the family of multi-configuration wavefunction based methods. In a nutshell, RASSCF subdivides the full active space (AS) into three subspaces: RAS1, with a fixed upper limit of holes; RAS2, where all possible permutations of electrons within the orbitals are considered; RAS3, with a maximal number of electrons. The possible configuration state functions (CSF's) over which the wavefunction is expanded, are built

according to these rules. A projection technique denoted *highly excited states* (HEXS) which selectively removes CSF's with a certain occupation from a given subspace is used to effectively project out undesired valence transitions preceding energetically the core transitions.[2]. The dynamical correlation missing at the RASSCF level is recovered through multireference second-order perturbation corrections (RASPT2).[3–5]

Below we outline the protocol for computing both linear and non-linear spectra. To speed up the calculations, we have taken advantage of the $C_{2h}$ symmetry of the molecule.

The AS is constructed as follows (Fig. S5).

- RAS1: contains both core-orbitals which are kept frozen to avoid orbital rotation during the variational optimization of the MO coefficients; the upper limit of holes is set to 2;
- RAS2: three $\pi-$type occupied orbitals are placed herein (one in irreducible representations A1 and two in B2)
- RAS3: 10 virtual orbitals are included (four, two, two and two in irreducible representations A1, A2, B1 and B2, respectively). The maximum of excitations in this sub-space was set to four.

In the following we designate the active space as RAS$(10, 2, 4; 2, 3, 10)$, where the first three indices denote the number of electrons, the upper limit of holes (in RAS1) and the upper limit of excitations (in RAS3), respectively; while the last three indies denotes the number of orbitals included in the three subspaces: in order, RAS1, RAS2 and RAS3.

The construction of the RAS3 space is vital for the completeness of the spectrum as every virtual orbital is potentially the source of a core-excited state and, consecutively, of a signal. Its composition was determined in the following way. First, preliminary calculations were run for each of the three symmetries A1, B1 and B2 (states of the A2 symmetry are not coupled to the GS) where up to ten virtual orbitals were included in the corresponding irreducible representation and up to 15 states were computed at the RASSCF/RASPT2 level[6]. Subsequently, the nature of the transitions comprising the carbon K-edge of the XANES spectrum up to 296 eV was analyzed in order to identify the virtual orbitals giving rise to the leading CSF's in the multiconfigurational wavefunctions involved in the identified transitions. The RAS$(10, 2, 4; 2, 3, 10)$ was constructed by limiting RAS3 to the virtual orbitals identified through the aforementioned analysis. Finally, it was verified that the results obtained with the RAS$(10, 2, 4; 2, 3, 10)$ reproduce the transitions identified previously.

The same RAS(10, 2, 4; 2, 3, 10) was utilized to obtain the $g$, $e$ and $f$ manifolds[7]. The GS was computed in a state-specific calculation. The $e$ manifold consisting of six states of A1, four states of B1 and three states of B2 symmetry was obtained by selectively removing all CSF's with a full (i.e. four electrons) occupation in the RAS1 subspace[8]. Finally, the $f$ manifold consisting of twelve states in each of the four symmetries of the $D_{2h}$ point group was obtained by removing all CSF's with four and three electrons in the RAS1 subspace. Thus, the total Hamiltonian is constructed of 62 electronic states: one GS, 13 single core-excitations and 48 double-core excitations. We note, that in the calculation of the GS and $f$ manifold orbital relaxation was restricted only within the active space when (thus effectively prohibiting rotations out of the AS) in order to preserve the composition of the AS. Benchmarking against calculation where the orbitals were allowed to relax freely. Figure S4 shows that this restriction does not affect the final spectra.

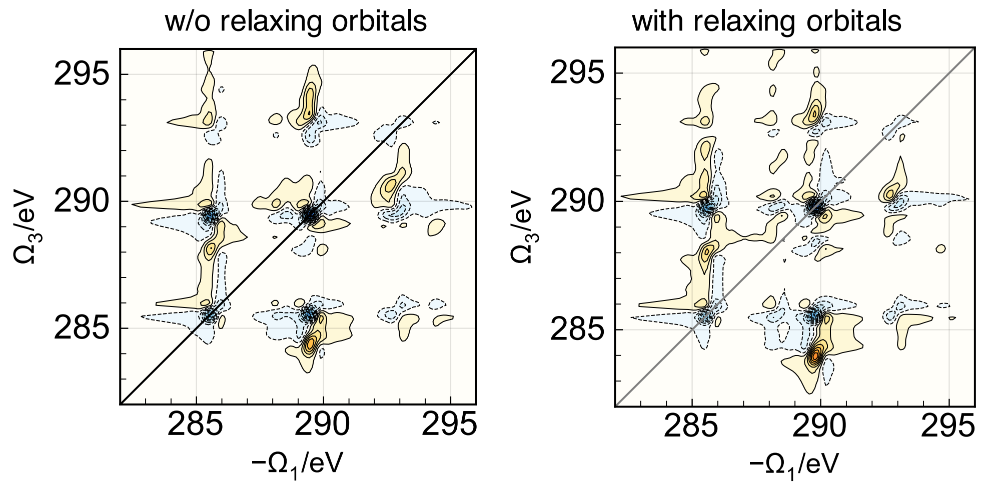


FIG. S4. Photon echo signal for 1,1-difluoroethylene when the orbitals in the active space are frozen (left) and when they are allowed to relax (right).

Multi state (MS)-RASPT2 was performed on top of each RASSCF calculation to account for the dynamical correlation, setting the ionization-potential electron-affinity shift [9, 10] of $0.0\,E_{\mathrm{h}}$. Core orbitals were explicitly correlated. To reduce problems with intruder states an imaginary shift [11] of $0.3\,E_{\mathrm{h}}$ has been applied.

Transition dipole moments between the $g$, $e$ and $f$ manifolds were computed by means of biorthogonalization through the RAS state interaction (SI) routine. The protocol is summarized in Fig. S3

Scalar relativistic effects have been included by using a second-order Douglas-Kroll-Hess Hamiltonian in combination with a relativistic atomic natural orbital basis set, ANO-RCC.[12] A triple-$\zeta$

basis function set augmented with two sets of $d$-functions for carbon and fluorine atoms and a set of $f$-functions for fluorine, thus giving rise to ANO-RCC: C[4s3p2d], F[4s3p2d1f], H[2s1p]. A density-fitting approximation of the electron repulsion integrals has been used, knows as Cholesky decomposition.[13]

All calculations were performed in the gas-phase with the OpenMolcas suite.[14, 15]

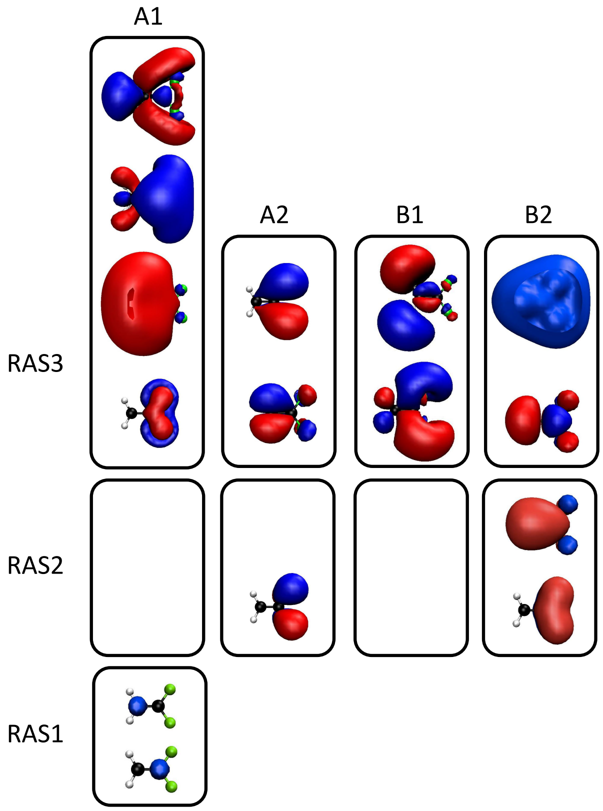


FIG. S5. Orbitals from the active space RAS(10; 2; 4; 2; 3; 10).

## S3. SIMULATIONS OF SPECTRA

The XAS, PE and DQC signals are calculated using the sum-over-states (SOS) protocol. The SOS formula for XAS is given below in Eq. (S9). Expressions for the 2D-PE and 2D-DQC can be derived similarly, details can be found in Ref. [16]. The lifetime broadening of the core-polariton is accounted for by a decay constant $\gamma_{ji} = 0.3\,\text{eV}$. We use attosecond pulses with central frequency around $\omega_j^0 = 288\,\text{eV}$ for all $j$ and bandwidth $15\,\text{eV}$ such that $E_j(\omega_j) \approx E_j(\omega_j^0)$ for $\omega \in (285, 296)$ eV. Such pulses can be generated by free-electron lasers [17]. All the interactions between external laser pulses and molecules are assumed in the perturbative regime.

The single-polariton and two-polariton states are computed by diagonalizing the polariton Hamiltonian represented in the direct-product electronic-photonic basis $|\alpha n\rangle \equiv |\alpha\rangle \otimes |n\rangle$ up to double excitations, where $\alpha$ denotes electronic state and $n$ is the photon number state. For XANES, we consider $N$ molecules and include the collective core-excited state $\{\ |\ E_{\alpha 0}0\rangle,\ |\ G1\rangle\ \}$. For 2D-PE and 2D-DQC spectra, we consider a single molecule and include $\left\{|f0\rangle\,, |e1\rangle\,, |g2\rangle\right\}$.

In the DQC simulations for $S(\Omega_2, \Omega_1; T_3)$, we focus on $T_3 \approx 0$. In practice, a very small number $\sim 1 \times 10^{-5}$as is used to avoid cancellation of the two diagrams at $T_3 = 0$. And similarly for $S(\Omega_3, \Omega_2; T_1)$.

### S3.A. Sum-over-states expression for XANES

We adopt a superoperator notation where the density matrix is written as a vector $\rho = \sum_{ij} \rho_{ij} \,|i\rangle \langle j| \to \sum_{ij} \rho_{ij} |ij\rangle\rangle$, and $\mathcal{V}_{\mathrm{L}}\rho \equiv V\rho$, $\mathcal{V}_{\mathrm{R}}\rho \equiv \rho V$ are, respectively, the left and right superoperators, $\mathcal{V}_{\pm}\rho \equiv [V, \rho]_{\pm}$ the commutator and anticommutator [18]. We assume a fixed polarization and suppress the vector notation of the dipole and electric fields.

X-ray absorption near edge structure (XANES) uses a single x-ray pulse

$$E(t) = \int_0^\infty \mathrm{d}\omega E(\omega) e^{-i\omega t} + \text{c.c.}. \tag{S5}$$

The Feynman diagram for XANES is shown in Fig. 1 and the corresponding expression reads

$$\langle V(t)\rangle = \int_0^\infty \mathrm{d}\tau \langle\langle V^\dagger | \mathcal{G}(\tau) \mathcal{V}_{\mathrm{L}}^\dagger | gg\rangle\rangle E(t-\tau) \tag{S6}$$

where $\mathcal{G}(t-t') = -i\theta(t-t')e^{-i\mathcal{L}(t-t')}$ with the Liouvillian $\mathcal{L}\rho = [H, \rho]$ is the Green's function for the Liouville-von Neumann equation. Inserting Eq. (S5) into Eq. (S6) leads to

$$\langle V(t)\rangle = \int_0^\infty \frac{\mathrm{d}\omega}{2\pi} \frac{\mu_{ge}\mu_{eg}}{\omega - \omega_{eg} + i\gamma_{eg}} E(\omega) e^{-i\omega t} = -i\theta(t)\mu_{eg}\mu_{ge} E(\omega_{eg} - i\gamma_{eg}) e^{-i\omega_{eg}t - \gamma_{eg}t} \tag{S7}$$

where $\omega_{ij} \equiv \omega_i - \omega_j$, $\mu_{ij}$ are respectively the transition energies, transition dipole moments for core-excitations without the cavity, and for core-polaritons inside the cavity. In the second equality in Eq. (S7), we have extended the lower integration limit to $-\infty$ since $E(\omega)$ is localized around a central frequency in the X-ray regime, and then used Cauchy's integral formula in the lower half circle. Inserting Eq. (S7) into the frequency-dispersed signal [19] (photon flux into each frequency photon mode)

$$S_{\mathrm{XAS}}(\omega) = -2\,\mathrm{Im}\,\langle V(\omega)\rangle\, E^*(\omega), \tag{S8}$$

where $\mathbf{V}(\omega) = \int_{-\infty}^{+\infty} \mathrm{d}t \mathbf{V}(t) e^{i\omega t}$ $(\mathbf{E}^*(\omega))$ is the Fourier transform of $\mathbf{V}(t)$ $(\mathbf{E}^*(t)$, the negative-frequency component of the electric field), leads to the sum-over-states expression

$$S_{\mathrm{XAS}}(\omega) = -2\,\mathrm{Im}\sum_e \frac{\mu_{eg}\mu_{ge}E(\omega_{eg} - i\gamma_{eg})E^*(\omega)}{\omega - \omega_{eg} + i\gamma_{eg}} \tag{S9}$$

## S4. TWO-PHOTON ABSORPTION

In two-photon absorption (TPA), the system is excited from the ground state to two-polariton states by simultaneously absorbing two photons. The TPA employs two laser pulses with electric field

$$E(t) = E_1 e^{-i\omega_1 t} + E_2 e^{-i\omega_2 t} + \text{c.c.}, \tag{S10}$$

and the signal can be defined as the transition rate to the final states $|f\rangle$, $S_{\mathrm{TPA}} = \lim_{t\to\infty} \sum_f \frac{\mathrm{d}P_f(t)}{\mathrm{d}t}$ where $P_f(t) = \mathrm{Tr}\left\{\rho(t)\,|f\rangle\,\langle f|\right\}$. The time-loop diagrams for TPA are shown in Fig. S6, and the expression is given by [20]

$$S_{\mathrm{TPA}} = \delta(\omega_f - \omega_1 - \omega_2)|E_1E_2|^2 \left| \sum_e \frac{\mu_{fe}\mu_{eg}}{\omega_1 - \omega_e + i\gamma_e} + \frac{\mu_{fe}\mu_{eg}}{\omega_2 - \omega_e + i\gamma_e} \right|^2 \tag{S11}$$

where $e$ runs over the intermediate single-polariton states.

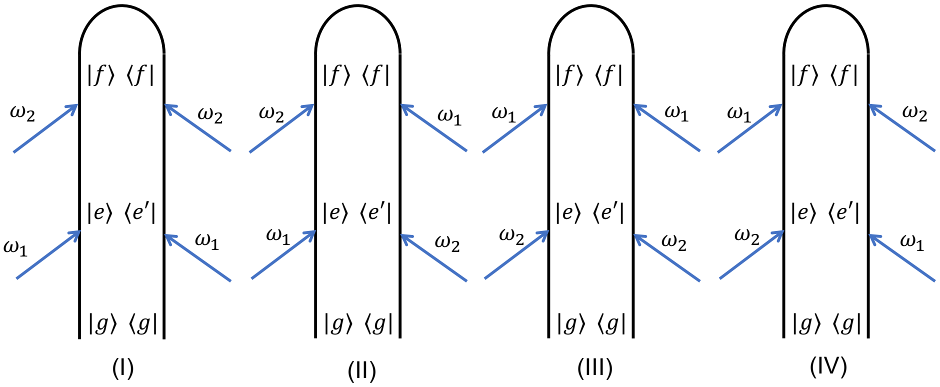


FIG. S6. Time-loop diagrams for the two-photon absorption signal. The four diagrams arise from the time-ordering of the four interactions along time-loop counterclockwise.

Figure S7 shows the TPA spectra $S_{\mathrm{TPA}}(\omega_1 + \omega_2, \omega_1)$ for bare molecules and for the core-polaritons. The peaks show the correlation between the bipolariton states $|f\rangle$ and the single-polariton states $|e\rangle$. The y-axis shows the bipolariton resonances $\omega_{fg}$ and the x-axis shows the transition energy either between the single-polariton and the ground state $\omega_{eg}$ or between the

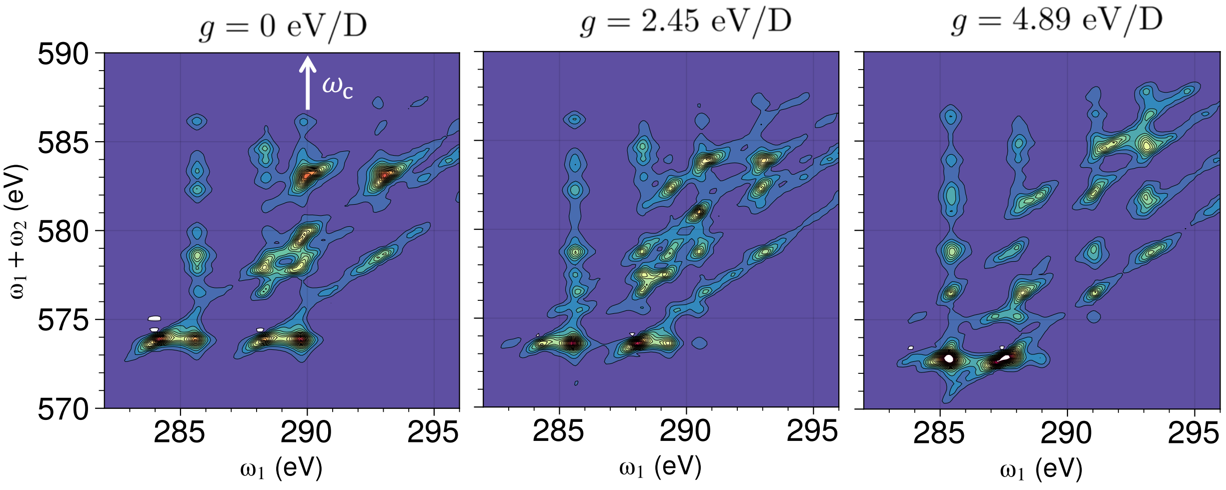


FIG. S7. Two-photon absorption spectra $S_{\mathrm{TPA}}(\Omega_1 + \omega_2, \Omega_1)$ for (a) bare molecule and for (b,c) core-polaritons of 1,1-difluoroethylene in an X-ray cavity. Here $\omega_c = 290\,\mathrm{eV}$, and the coupling strength $g$ is indicated.

bipolariton state and the single-polariton state $\omega_{fe}$. The latter corresponds to the system absorbing $\omega_2$ first and then absorbing $\omega_1$ to the final state. The TPA spectra provide similar information as the double quantum coherence signal


[1] Per-Åke Malmqvist, Alistair. Rendell, and Björn O. Roos, "The restricted active space self-consistent-field method, implemented with a split graph unitary group approach," The Journal of Physical Chemistry **94**, 5477–5482 (1990).

[2] Marcus Lundberg and Micka el G. Delcey, *Transition Metals in Coordination Environments*, edited by Ewa Broclawik, Tomasz Borowski, and Mariusz Radoń (Springer International Publishing, 2019) Chap. Multiconfigurational Approach to X-ray Spectroscopy of Transition Metal Complexes.

[3] K. Andersson, P. Å Malmqvist, B. O. Roos, A. J. Sadlej, and K. Wolinski, J. Phys. Chem. **94**, 5483–5488 (1990).

[4] V. Sauri, L. S. Andres, A. R. M. Shahi, L. Gagliardi, S. Vancoillie, and K. Pierloot, J. Chem. Theory Comput. **7**, 153 (2011).

[5] Daniel Roca-Sanjuán, Francesco Aquilante, and Roland Lindh, "Multiconfiguration second-order perturbation theory approach to strong electron correlation in chemistry and photochemistry," Wiley Interdisciplinary Reviews: Computational Molecular Science **2**, 585–603 (2011).

[6] Details on the RASPT2 parameters are given below.

[7] The use of a uniform AS for all manifolds is a requirement for computing the transition dipole moments $\mu_{eg}$ and $\mu_{fe}$.

[8] Note that the states belonging to each irreducible representation have to be computed in a separate state-average calculation.

[9] Giovanni Ghigo, Björn O. Roos, and Per-Åke Malmqvist, "A modified definition of the zeroth-order hamiltonian in multiconfigurational perturbation theory (caspt2)," Chem. Phys. Lett. **396**, 142 – 149 (2004).

[10] J. Patrick Zobel, Juan J. Nogueira, and Leticia González, "The IPEA dilemma in CASPT2," Chemical Science **8**, 1482–1499 (2017).

[11] Niclas Forsberg and Per-Åke Malmqvist, "Multiconfiguration perturbation theory with imaginary level shift," Chem. Phys. Lett. **274**, 196 – 204 (1997).

[12] Björn O. Roos, Valera Veryazov, and Per-Olof Widmark, "Relativistic atomic natural orbital type basis sets for the alkaline and alkaline-earth atoms applied to the ground-state potentials for the corresponding dimers," Theor. Chem. Acc. **11**, 2004 (345).

[13] F. Aquilante, T. B. Pedersen, and R. Lindh, Theor. Chem. Acc. **124**, 1 (2009).

[14] Ignacio Fdez. Galván, Morgane Vacher, Ali Alavi, Celestino Angeli, Francesco Aquilante, Jochen Autschbach, Jie J. Bao, Sergey I. Bokarev, Nikolay A. Bogdanov, Rebecca K. Carlson, Liviu F. Chibotaru, Joel Creutzberg, Nike Dattani, Mickaël G. Delcey, Sijia S. Dong, Andreas Dreuw, Leon Freitag, Luis Manuel Frutos, Laura Gagliardi, Frédéric Gendron, Angelo Giussani, Leticia González, Gilbert Grell, Meiyuan Guo, Chad E. Hoyer, Marcus Johansson, Sebastian Keller, Stefan Knecht, Goran Kovačević, Erik Källman, Giovanni Li Manni, Marcus Lundberg, Yingjin Ma, Sebastian Mai, João Pedro Malhado, Per Åke Malmqvist, Philipp Marquetand, Stefanie A. Mewes, Jesper Norell, Massimo Olivucci, Markus Oppel, Quan Manh Phung, Kristine Pierloot, Felix Plasser, Markus Reiher, Andrew M. Sand, Igor Schapiro, Prachi Sharma, Christopher J. Stein, Lasse Kragh Sø rensen, Donald G. Truhlar, Mihkel Ugandi, Liviu Ungur, Alessio Valentini, Steven Vancoillie, Valera Veryazov, Oskar Weser, Tomasz A. Weso?owski, Per-Olof Widmark, Sebastian Wouters, Alexander Zech, J. Patrick Zobel, and Roland Lindh, "Openmolcas: From source code to insight," Journal of Chemical Theory and Computation **15**, 5925–5964 (2019).

[15] Francesco Aquilante, Jochen Autschbach, Alberto Baiardi, Stefano Battaglia, Veniamin A. Borin, Liviu F. Chibotaru, Irene Conti, Luca De Vico, Mickaël Delcey, Ignacio Fdez. Galván, Nicolas Ferré, Leon Freitag, Marco Garavelli, Xuejun Gong, Stefan Knecht, Ernst D. Larsson, Roland Lindh, Marcus Lundberg, Per Åke Malmqvist, Artur Nenov, Jesper Norell, Michael Odelius, Massimo Olivucci, Thomas B. Pedersen, Laura Pedraza-González, Quan M. Phung, Kristine Pierloot, Markus Reiher, Igor Schapiro, Javier Segarra-Martí, Francesco Segatta, Luis Seijo, Saumik Sen, Dumitru-Claudiu Sergentu, Christopher J. Stein, Liviu Ungur, Morgane Vacher, Alessio Valentini, and Valera Veryazov, "Modern quantum chemistry with [open]molcas," The Journal of Chemical Physics **152**, 214117 (2020).

[16] Markus Kowalewski, Benjamin P. Fingerhut, Konstantin E. Dorfman, Kochise Bennett, and Shaul Mukamel, "Simulating Coherent Multidimensional Spectroscopy of Nonadiabatic Molecular Processes: From the Infrared to the X-ray Regime," Chem. Rev. **117**, 12165–12226 (2017).

[17] C. Pellegrini, A. Marinelli, and S. Reiche, “The physics of x-ray free-electron lasers,” Rev. Mod. Phys. **88**, 015006 (2016).

[18] Konstantin E. Dorfman and Shaul Mukamel, “Nonlinear spectroscopy with time- and frequency-gated photon counting: A superoperator diagrammatic approach,” Phys. Rev. A **86**, 013810 (2012).

[19] Markus Kowalewski and Shaul Mukamel, “Manipulating molecules with quantum light,” Proc. Natl. Acad. Sci. **114**, 3278–3280 (2017).

[20] Bing Gu and Shaul Mukamel, “Manipulating Two-Photon-Absorption of Cavity Polaritons by Entangled Light,” J. Phys. Chem. Lett. **11**, 8177–8182 (2020).
